# Supplementary material for: Inverse Design of Multi-band Reflective Polarizing Metasurfaces Using Generative Machine Learning
Source: arXiv:2207.04019 source file (2022-07-08)
Supplement: Supplementary file 1 [file Additional.tex]

\section*{Additional information}

To include, in this order: \textbf{Accession codes} (where applicable); \textbf{Competing interests} (mandatory statement). 

The corresponding author is responsible for submitting a \href{http://www.nature.com/srep/policies/index.html#competing}{competing interests statement} on behalf of all authors of the paper. This statement must be included in the submitted article file.
